# Supplementary material for: GenURL: A General Framework for Unsupervised Representation Learning
Source: arXiv:2110.14553 source file (2024-04-16)
Supplement: Supplementary file 1 [file ch7_appendix.tex]

\appendix
\section{Appendix}
\label{app}
We first provide detailed implementation settings for self-supervised visual representation learning (SSL), knowledge distillation (KD), graph embedding (GE), and dimension reduction (DR) tasks in \ref{app:implement}. Then, additional ablation studies of GenURL are detailed in \ref{app:ablation} and future work of GenURL is discussed in \ref{app:impact}.

% fig: visualization SSL
\begin{figure*}[h]
    \centering
    \includegraphics[width=0.98\linewidth]{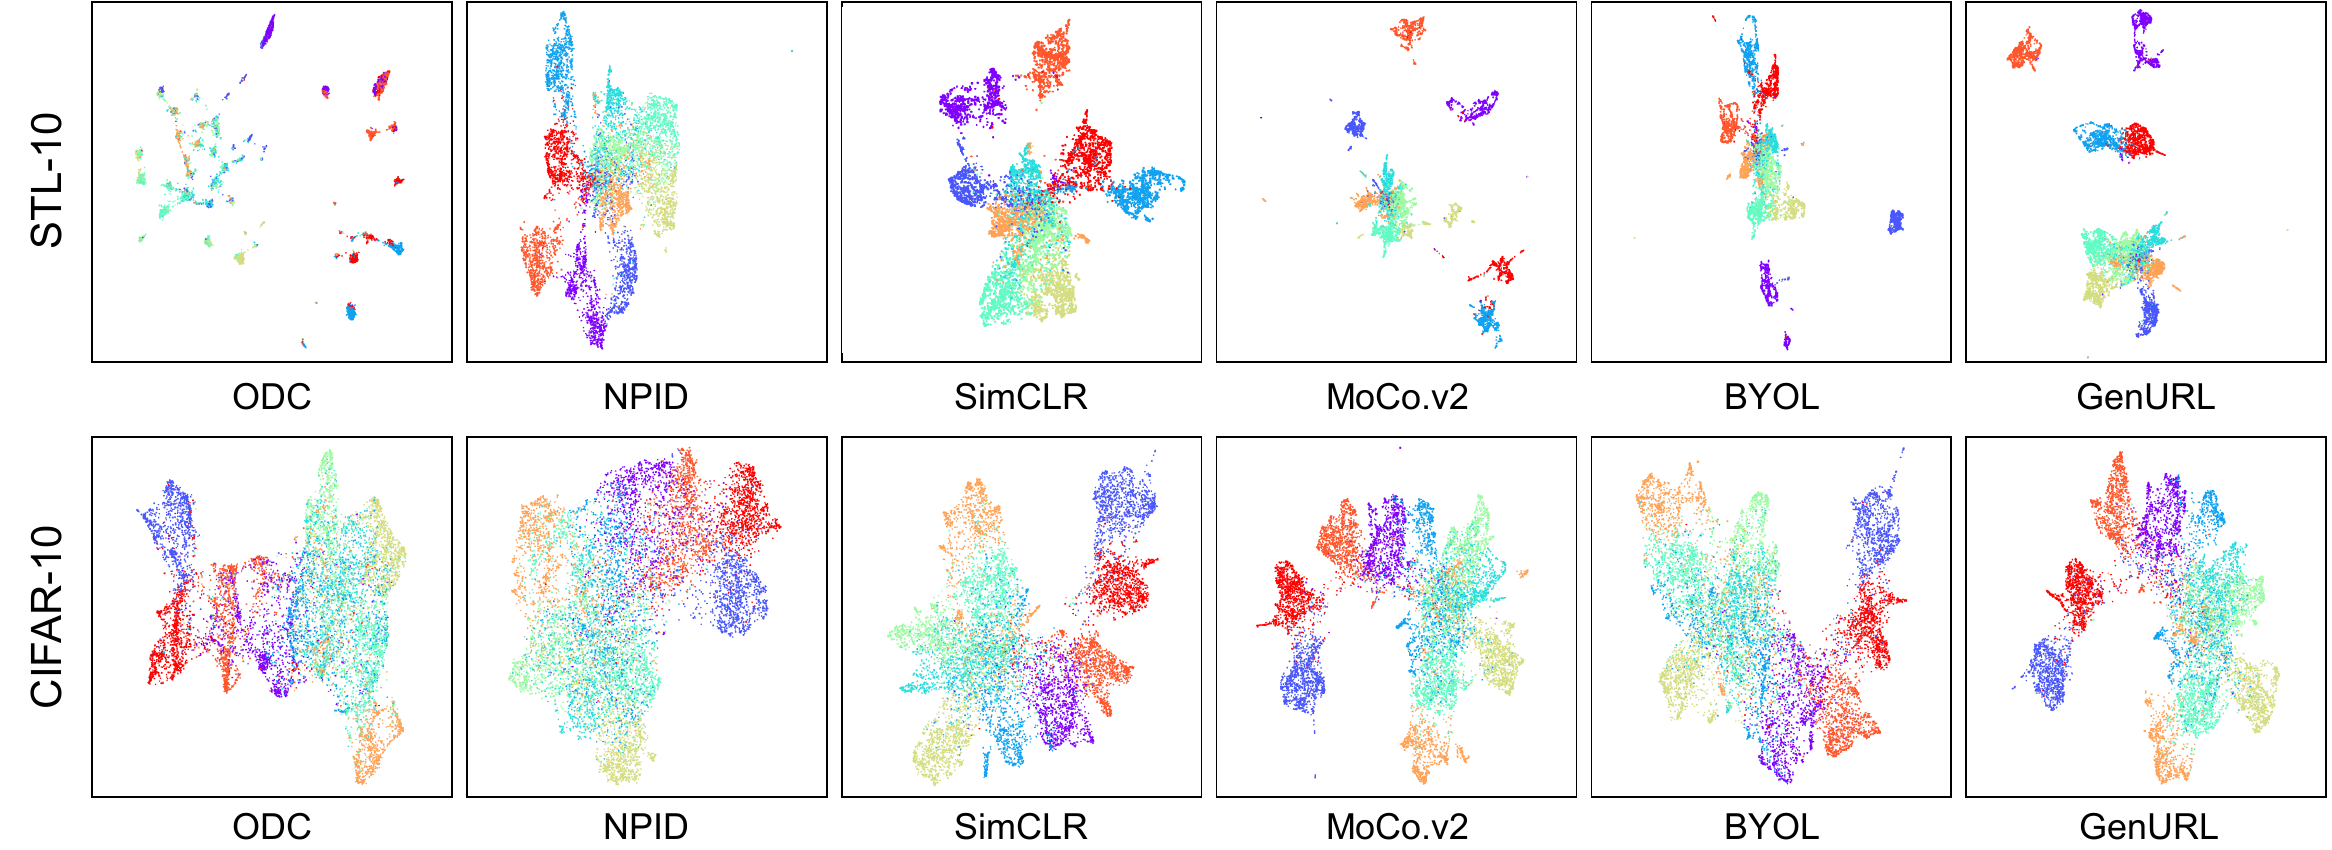}
    \caption{Visualization of the latent space learned by various SSL methods on STL-10 and CIFAR-10. ResNet-50 is adopted as the encoder with 800-epoch pre-training. Compared to contrastive-based methods, GenURL preserves the geometric structures of clusters while yielding clear distinctions between every two clusters.}
    \label{fig:app_SSL_STL_CIFAR}
    \vspace{-10pt}
\end{figure*}

\subsection{Implement Details}
\label{app:implement}
\paragraph{Self-supervised learning.}
We follow MoCo.v2~\cite{2020mocov2} for contrastive learning (CL) pre-training, which adopts ResNet encoder with a two-layer MLP projector. All contrastive learning methods adopt the same network and augmentation settings, while other methods use default settings in their paper. The data augmentation setting in MoCo.v2 is as follows: Geometric augmentations include \textit{RandomResizedCrop} with the scale in $[0.2,1.0]$ and \textit{RandomHorizontalFlip}. Color augmentation include \textit{ColorJitter} with \{brightness, contrast, saturation, hue\} strength of $\{0.4, 0.4, 0.4, 0.1\}$ with an applying probability of $0.8$, and \textit{RandomGrayscale} with an applying probability of $0.2$. Blurring augmentation uses a Gaussian kernel of size $23\times 23$ with a standard deviation uniformly sampled in $[0.1, 2.0]$. As shown in Table.9, we use $\nu_{X} = \nu_{Z}=100$ and $\sigma_{X}=\sigma_{Z}=0.1$ for GenURL on CIFAR-10, CIFAR-100, STL-10, Tiny ImageNet, and ImageNet-1k.

\paragraph{Knowledge distillation.}
In the KD task, GenURL follows the settings of the current-proposed contrastive-based KD method SEED~\cite{iclr2021seed}, which adopts the non-linear projector network and data augmentations used in MoCo.V2. Similar to the SSL task, GenURL uses $\nu_{X} = \nu_{Z} = 100$ and $\sigma_{X}=1$.

\paragraph{Graph embedding.}
In the GE tasks, basic information of datasets and most hyper-parameters in GenURL is in Table.10. We adopt $L_{2}$ distance with $\sigma_{Z}=1$ and tune various hyper-parameters as follows. As for $\mu$ and $\sigma$, we perform grid search of $\mu_{Z}$ and $\sigma_{Z}$ for the latent space in ${1e-2, 1e-1, 1, 1e1, 1e2}$ on the validation set. As for $\mu_{i,2}$ and $\sigma_{2}$ of the raw attribute space, we use a binary search (requires $O(n^{2})$) with $5$ nearest neighbors for each data point, \textit{i.e.}, the optimal hyper-parameters guarantee the $5$ nearest neighbors of $x_{i}$ have a large similarity score. There are similar practices in UMAP~\cite{2018UMAP} and t-SNE~\cite{jmlr2008tSNE}. If the dataset is too large, we set $\mu_{i,2}$ and $\sigma_{2}$ to the statistic mean and std of the whole dataset.

\paragraph{Dimension reduction.}
Similar to the GE task setting, GenURL performs DR tasks with the kNN graph built on the input $X$. We set $\nu_{Z}=0.01$ and $\sigma_{X}$ to $5$ and $20$ for MNIST and FMNIST respectively.

\subsection{More Ablation}
\label{app:ablation}
In the SSL task, most CL methods need long training to reach convergence. We conduct additional ablation studies to verify the convergence speed of GenURL on STL-10 with ResNet-50 (using the same setting as Sec.4.1). We first train SimCLR and MoCo.v2 with two different batch size settings to verify whether using a small batch size is helpful to the convergence speed. Then, we adopt a binary mask of size $B\times B$ to similarity matrixes in GenURL (in Eq.\ref{eq:final_loss}) to randomly stop calculating some parts of pairwise distance in a mini-batch, where $B$ denotes the batch size. The binary mask is generated randomly and only affects non-eye positions. As shown in Table.11, GenURL has faster convergence speeds and achieves the best performance with more pairwise distance when all methods adopt a small batch size.

% image datasets

\begin{table}[H]
\centering
\resizebox{1.0\columnwidth}{!}{
    \begin{tabular}{lccccc}
    \toprule
    Dataset       & Tasks   & Train   & Test & Resolution     & Class \\ \hline
    MNIST         & DR      & 50k     & 10k  & 28$\times$28   & 10      \\
    FMNIST        & DR      & 50k     & 10k  & 28$\times$28   & 10      \\
    CIFAR-10      & SSL     & 50k     & 10k  & 32$\times$32   & 10      \\
    CIFAR-100     & SSL     & 50k     & 10k  & 32$\times$32   & 100     \\
    STL-10        & SSL, KD & 5k+100k & 8k   & 96$\times$96   & 10      \\
    Tiny-ImageNet & SSL     & 100k    & 10k  & 64$\times$64   & 200     \\
    ImageNet-1k   & SSL     & 1.28M   & 5k   & 224$\times$224 & 1k      \\
    \bottomrule
    \end{tabular}}
    \caption{Basic information of image datasets.}
    \label{tab:app_img_dataset}
\end{table}

\vspace{-10pt}
% graph datasets

\begin{table}[H]
\centering
\resizebox{.90\columnwidth}{!}{
    \begin{tabular}{lcccccc}
    \toprule
             & Nodes  & Features & Edges  & Class   & $\nu_{Z}$ & $\alpha_2$ \\ \hline
    CORA     & 2,708  & 1,433    & 5,429  & 7       & 0.001     & 1.0        \\
    CiteSeer & 3,327  & 3,703    & 4,732  & 6       & 0.005     & 0.5        \\
    PubMed   & 19,717 & 500      & 44,338 & 3       & 0.003     & 50         \\
    \bottomrule
    \end{tabular}}
    \caption{Basic information and GenURL hyper-parameters of graph datasets.}
    \label{tab:app_ge_dataset}
\end{table}

\vspace{-10pt}
% table: ablation on ssl

\begin{table}[H]
\centering
\resizebox{.95\columnwidth}{!}{
    \begin{tabular}{lccc}
    \toprule
    Method         & batch      & 400ep             & 800ep        \\
                   & size       & Top1, Top 5       & Top1, Top 5  \\ \hline
    SimCLR         & 256        & 82.90, 99.26      & 86.61, 99.30 \\
    SimCLR         & 4096       & 86.92, 99.41      & 89.68, 99.66 \\
    MoCo.v2        & 256        & 84.89, 99.41      & 89.58, 99.30 \\
    MoCo.v2        & 1024       & 84.21, 98.30      & 88.95, 99.14 \\
    GenURL (100\%) & 256        & \bf{88.35, 99.25} & \bf{90.82, 99.41} \\
    GenURL (75\%)  & 256        & 87.86, 99.73      & 89.82, 99.26 \\
    GenURL (50\%)  & 256        & 86.44, 99.16      & 89.05, 99.10 \\
    GenURL (25\%)  & 256        & 85.29, 98.79      & 87.64, 99.57 \\
    \bottomrule
    \end{tabular}}
    \caption{Ablation of convergence speed of GenURL and CL methods on STL-10.}
    \label{tab:app_ablation}
\end{table}

\subsection{Analysis and Discussion}
\label{app:discussion}
We provide an extensive analysis of the hyper-parameters and loss functions in GenURL across different URL tasks to reflect the characteristics of various tasks.
Basically, we compare the results using different batch sizes, $\nu_{Z}$, $\sigma$, and loss functions for GenURL.

% figure: DR + GE ablation
\begin{figure}[b]
    \vspace{-8pt}
    \centering
    \includegraphics[width=1.0\linewidth]{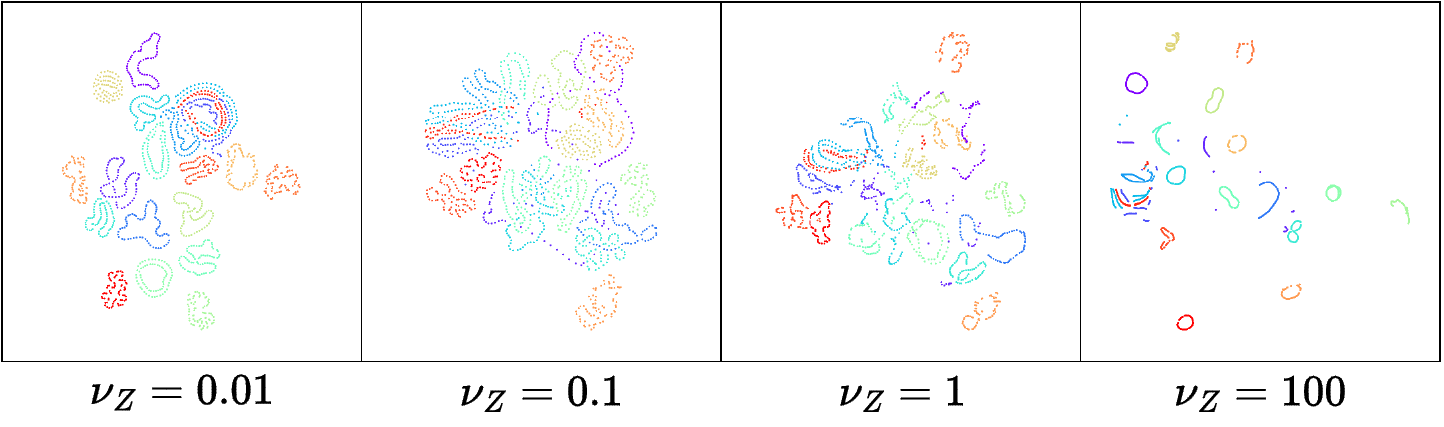}
\end{figure}
\begin{figure}[b]
    \vspace{-8pt}
    \centering
    \includegraphics[width=1.0\linewidth]{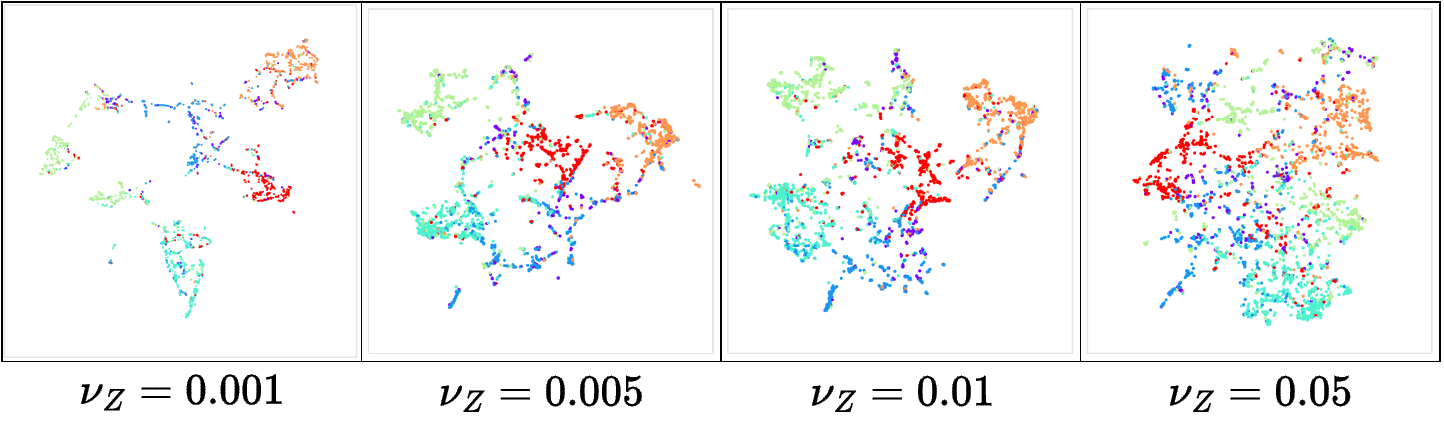}
    \vspace{-14pt}
    \caption{\textit{First row}: ablation of $\nu_{Z}$, $\sigma$ and batch size of the DR tasks on MNIST. \textit{Second row}: visuaization of learned embeddings using various $\nu_{Z}$ of the GE task on CiteSeer.}
    \label{fig:ge_dr_ablation}
    % \vspace{-8pt}
\end{figure}

% \vspace{-8pt}
\paragraph{Relationship between SSL and KD.}
% 验证采用GKL+self-distillation(KD)可以较好的解决SSL(离散空间的embedding问题)
We study the relationship between SSL and KD tasks to show that GenURL and loss functions can deal with the negative samples efficiently. Firstly, we first study the hyper-parameters to show the influence of choosing different $\nu_{Z}$ and $\sigma$. 
We follow the experiment settings in Sec.~\ref{ch5.1:ssl} and Sec.~\ref{ch5.2:KD}, and we compare the ablation results of SSL and KD on STL-10, as shown in Figure~\ref{fig:kd_ablation}. We find that GenURL prefers the similar $\nu_{Z}$ and $\sigma$ for both SSL and KD tasks, which indicates using $\nu_{Z}=100$ and $\sigma=1$, \textit{i.e.}, the standard Gaussian kernel, is suitable for $L_2$-normalized cosine distance. As for the batch size, most existing CL methods require a large batch size to keep enough contrastive examples~\cite{2020simclr, nips2020byol}. We notice that GenURL prefers small batch sizes like $256$ for the SSL task (suffering performance drops when the batch size increases) while prefers larger batch sizes for the KD task. It might be because pair-wise similarities of negative samples in SSL tasks are unreliable while regarded as dark knowledge in the KD task.~\cite{nips2014kd, iclr2021seed}. 
At the early training stage of the SSL task, the gradient from negative pairs might overwhelm positive samples, while in the KD task, negative samples are well-defined by the teacher model. 
Then, we evaluate the loss functions to verify our assumptions. Table~\ref{tab:ssl_loss_ablation} shows the linear evaluation results of using MSE, BCE, and GKL loss with different $p_{X}$ in SSL tasks, and Table~\ref{tab:kd_loss_ablation} shows the results of using MSE, BCE and GKL loss in KD tasks. We find that using the \textit{dynamic} version and the GKL loss in SSL tasks yield the best performance while using the large batch size, and the BCE loss in KD tasks performs better. We can conclude that using GKL with the \textit{dynamic} structural modeling can alleviate the negative effects of unreliable metric spaces.

% figure: DR and SSL
\begin{figure}[t]
    \centering
    \includegraphics[width=1.0\linewidth]{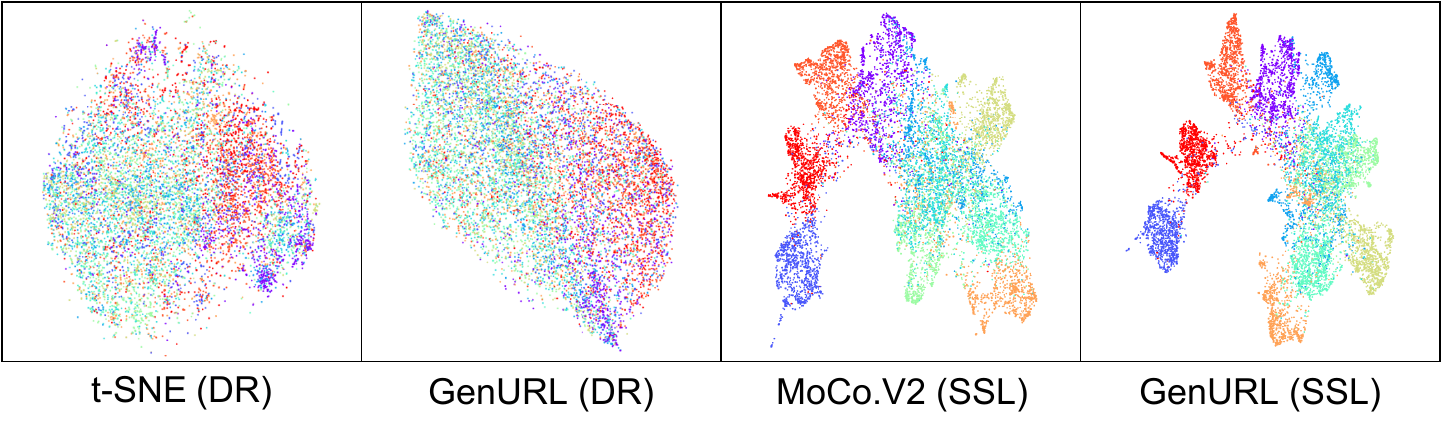}
    % \caption{Visualization of the learned representation with DR and SSL methods on CIFAR-10.}
    % \label{fig:SSL_DR2SSL_CIFAR_plot}
\end{figure}
\begin{figure}[t]
    \vspace{-8pt}
    \centering
    \includegraphics[width=1.0\linewidth]{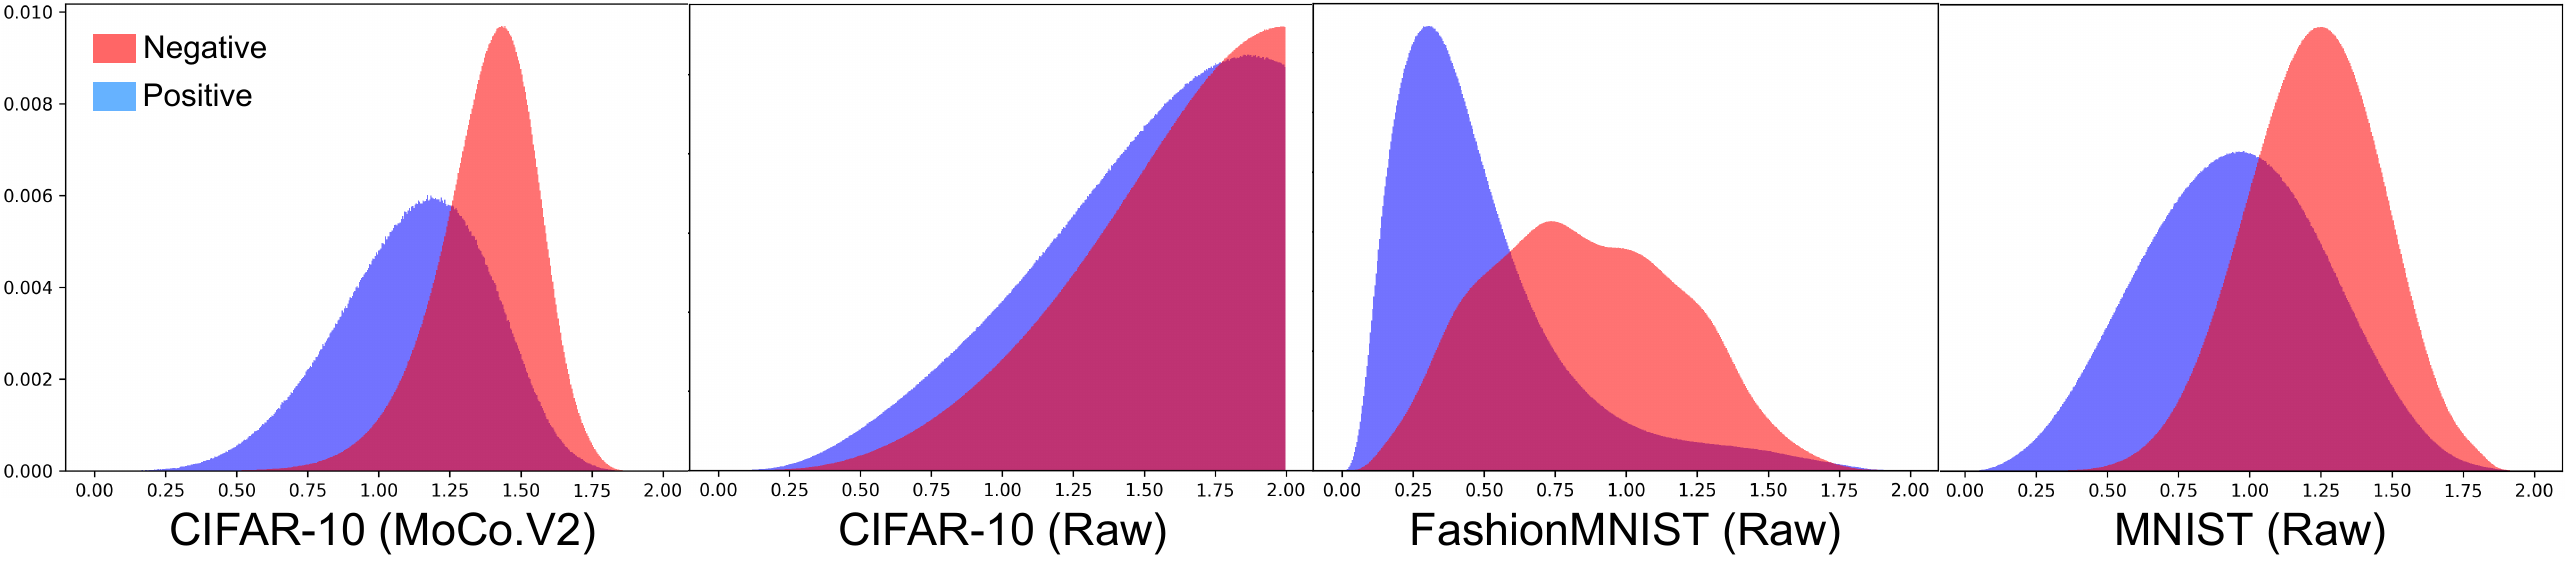}
    % \vspace{-12pt}
    \caption{Analysis of relationships of the SSL, KD, and DR tasks. \textit{First row}: visualization of learned embeddings on CIFAR-10. \textit{Second row}: histograms of the pair-wise cosine distance of the positive (blue) and negative pairs (red) on STL-10, CIFAR-10, and MNIST. Note that MoCo.v2 and raw denote the distance on the latent space (MoCo.v2) and raw feature spaces.}
    \label{fig:SSL_CIFAR_plot}
    \vspace{-8pt}
\end{figure}

% \vspace{-8pt}
\paragraph{Relationship between SSL and DR.}
We further discuss the relation between SSL and DR tasks (the \textit{dynamic} and \textit{static} $\tilde p_{X}$) with GenURL to explain the intrinsic or desired structures of data in URL tasks. 
Firstly, we study the effects of hyper-parameters in GenURL on both DR and SSL tasks. As shown in Figure~\ref{fig:ge_dr_ablation}, GenURL prefers smaller $\nu_{Z}$ for both tasks since the large $\nu_{Z}$ yields crowd embedding and the small $\nu_{Z}$ for more separable results. As for the DR task, GenURL produces the best representation with $\nu=0.001$, $\sigma=1$ to preserve more global relation between two distant sample pairs. 
Then, as shown in Figure~\ref{fig:SSL_CIFAR_plot}, we compare visualization of the learned representations with the DR and SSL methods on CIFAR-10. We find that SSL results (using the instance discrimination prior knowledge in SSL tasks) are more useful to downstream tasks like clustering and classification. We try to explain the difference between the DR and SSL tasks by computing the pair-wise distance between raw input samples and the latent space of teacher model, as shown in Figure~\ref{fig:SSL_CIFAR_plot}. We find that the input space is discriminative and reliable enough on MNIST and FMNIST for the DR task while is unreliable on CIFAR-10.

\subsection{Limitation and Future work}
\label{app:impact}
As for the societal impacts of GenURL, it can be regarded as a unified framework for the unsupervised representation learning (URL) problem that bridges the gap between various methods. The ablation studies of basic hyper-parameters can reflect the relationship between different URL tasks. The core idea in GenURL is to explore intrinsic structures of the data (the raw input space or empirical metric space) and preserve these structures in the latent space, which might inspire some improvements in various URL tasks. For example, the \textit{dynamic} $\widetilde p_{X}$ is similar to the hard negative mining problem in the SSL task~\cite{2021iclrHCL}.

As for the limitations of GenURL, we can conclude three aspects: (i) the proposed framework is relied on offline hyper-parameter tuning to adapt to new URL tasks, which makes it tough to handle more than two input similarities, (ii) GenURL cannot deal with the case of discrete empirical spaces well, \textit{e.g.}, the SSL tasks, and the \textit{dynamic} $\widetilde p_{X}$ should be improved in the future work, (iii) the performance of GenURL is still limit by negative samples (sensitive to the size of datasets and the batch size).
